# Supplementary material for: A Morphology Focused Diffusion Probabilistic Model for Synthesis of Histopathology Images
Source: arXiv:2209.13167 source file (2022-09-29)
Supplement: Supplementary file 1 [file appendix.tex]

\onecolumn

\appendix

\section{Input data}
\begin{figure}[ht]
\rotatebox[origin=c]{90}{\bfseries IDHC\strut}
\begin{subfigure}{.17\textwidth}
  \centering
  % include first image
  \includegraphics[width=\textwidth]{figs/512_IDHC_1.png} 
\end{subfigure}
\begin{subfigure}{.17\textwidth}
  \centering
  % include second image
  \includegraphics[width=\textwidth]{figs/512_IDHC_2.png}
\end{subfigure}
\begin{subfigure}{.17\textwidth}
  \centering
  % include third image
  \includegraphics[width=\textwidth]{figs/512_IDHC_3.png}  
\end{subfigure}
\begin{subfigure}{.17\textwidth}
  \centering
  % include fourth image
  \includegraphics[width=\textwidth]{figs/512_IDHC_4.png}  
\end{subfigure}
\begin{subfigure}{.17\textwidth}
  \centering
  % include fifth image
  \includegraphics[width=\textwidth]{figs/512_IDHC_5.png}  
\end{subfigure}
\newline
\rotatebox[origin=c]{90}{\bfseries IDHNC\strut}
\begin{subfigure}{.17\textwidth}
  \centering
  % include first image
  \includegraphics[width=\textwidth]{figs/512_IDHNC_1.png} 
\end{subfigure}
\begin{subfigure}{.17\textwidth}
  \centering
  % include second image
  \includegraphics[width=\textwidth]{figs/512_IDHNC_2.png}
\end{subfigure}
\begin{subfigure}{.17\textwidth}
  \centering
  % include third image
  \includegraphics[width=\textwidth]{figs/512_IDHNC_3.png}  
\end{subfigure}
\begin{subfigure}{.17\textwidth}
  \centering
  % include fourth image
  \includegraphics[width=\textwidth]{figs/512_IDHNC_4.png}  
\end{subfigure}
\begin{subfigure}{.17\textwidth}
  \centering
  % include fifth image
  \includegraphics[width=\textwidth]{figs/512_IDHNC_5.png}  
\end{subfigure}
\newline
\rotatebox[origin=c]{90}{\bfseries IDHWT\strut}
\begin{subfigure}{.17\textwidth}
  \centering
  % include first image
  \includegraphics[width=\textwidth]{figs/512_IDHWT_1.png} 
\end{subfigure}
\begin{subfigure}{.17\textwidth}
  \centering
  % include second image
  \includegraphics[width=\textwidth]{figs/512_IDHWT_2.png}
\end{subfigure}
\begin{subfigure}{.17\textwidth}
  \centering
  % include third image
  \includegraphics[width=\textwidth]{figs/512_IDHWT_3.png}  
\end{subfigure}
\begin{subfigure}{.17\textwidth}
  \centering
  % include fourth image
  \includegraphics[width=\textwidth]{figs/512_IDHWT_4.png}  
\end{subfigure}
\begin{subfigure}{.17\textwidth}
  \centering
  % include fifth image
  \includegraphics[width=\textwidth]{figs/512_IDHWT_5.png}  
\end{subfigure}
\caption{Selection of patches with size = 512x512 pixels extracted from the TCGA dataset\cite{dataset}. Each row represents a class.}
\label{fig:extracted}
\end{figure}

\begin{table}[h]
\centering
\setlength{\tabcolsep}{10pt}
%\setlength{\tabcolsep}{7pt}
%\setlength{\tabcolsep}{2em}

%\tiny
\begin{tabular}{l|llll}
patch size & IDHC & IDHNC & IDHWT & Total \\
\hline
512x512 & 10396 & 14310 & 3296 & 28002 \\
128x128 & 12139 & 16975 & 4663 & 33777\\
64x64 & 298 & 1090 & 588 & 1967\\
\end{tabular}
\caption{Number of patches for every patch size used in this paper.}
\label{tab:number-of-patches}
\end{table}
\newpage
\section{Model parameters}
\begin{table}[h]
\centering
\setlength{\tabcolsep}{10pt}
%\setlength{\tabcolsep}{7pt}
%\setlength{\tabcolsep}{2em}

%\tiny
\begin{tabular}{l|lllll}
\hline
 & DPM1 & DPM2 & DPM3 & DPM4 & DPM5\\
\hline
Image size & 512 & 512 & 512 & 64 & 128\\
Diffusion steps & 1000 & 1000 & 1000 & 1000 & 1000\\
Noise schedule & linear & linear & linear & linear & linear\\
Channels & 64 & 64 & 64 & 64 & 64\\
Heads & 4 & 4 & 4 & 4 & 4\\
Heads channels & 64 & 64 & 64 & 64 & 64\\
Attention resolution & 32,16,8 & 32,16,8 & 64 & 32,16,8 & 32,16,8\\
BigGAN up/downsample & yes & yes & yes & yes & yes\\
Dropout & 0.0 & 0.0 & 0.0 & 0.0 & 0.0\\
Batch size & 4 & 4 & 4 & 4 & 4\\
Learning rate & 1e-4 & 1e-4 & 1e-4 & 1e-4 & 1e-4\\
Weighting scheme & standard & P2 & P2 & P2 & P2\
\end{tabular}
\caption{Hyperparameters for diffusion probabilistic models used in this paper.}
\label{tab:model-hyperparameters}
\end{table}

\section{Results}
\begin{figure*}[h]
\begin{subfigure}{\textwidth}
  \centering
  % include first image
  \includegraphics[width=0.2\textwidth]{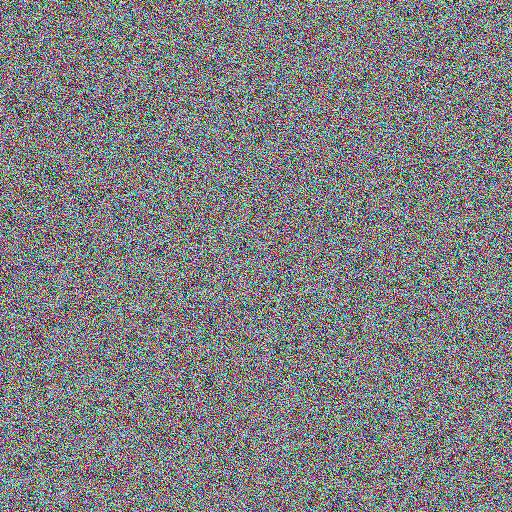} 
\end{subfigure}
\caption{Synthetic image generated with DPM3.}
\label{fig:images-DPM3}
\end{figure*}

\begin{figure*}[h]
\begin{subfigure}{\textwidth}
  \centering
  % include first image
  \includegraphics[width=0.2\textwidth]{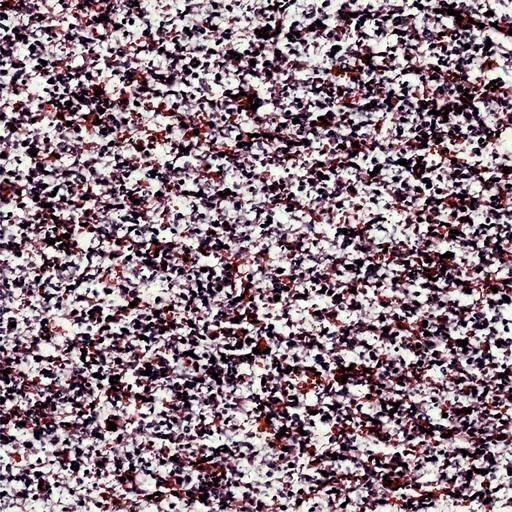} 
  % include second image
  \includegraphics[width=0.2\textwidth]{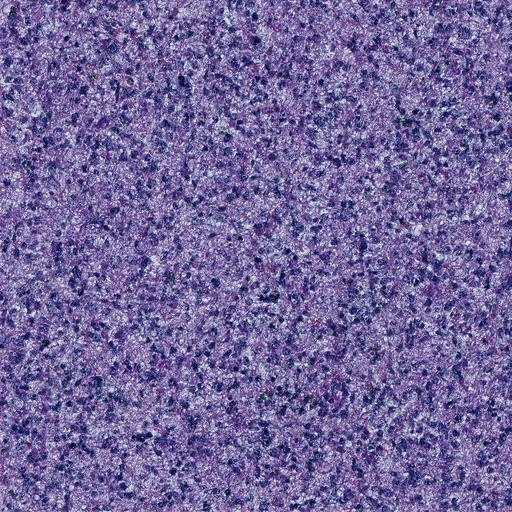}
  % include third image
  \includegraphics[width=0.2\textwidth]{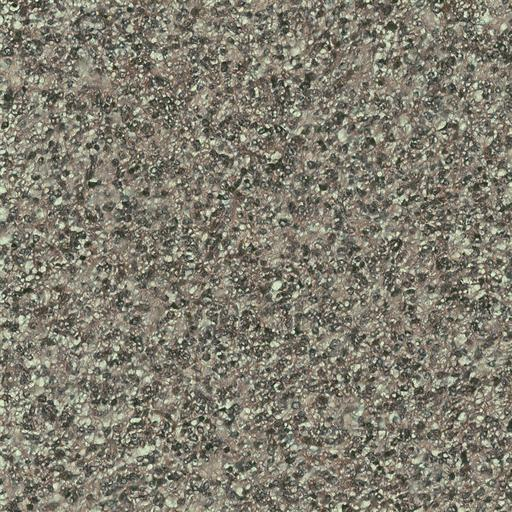} 
  % include fourth image
  \includegraphics[width=0.2\textwidth]{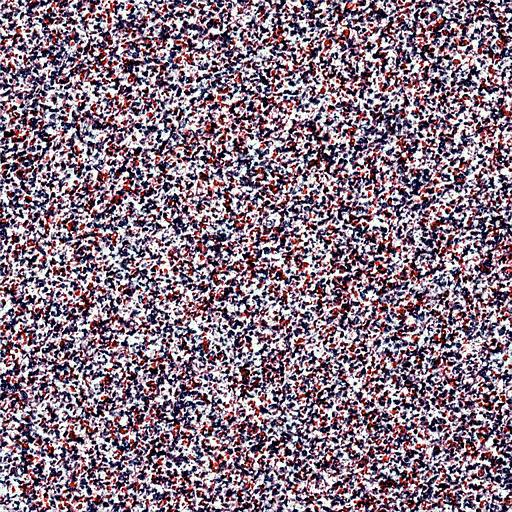}
\end{subfigure}
\caption{Synthetic images generated with DPM1.}
\label{fig:images-DPM1}
\end{figure*}

\begin{figure*}[h]
\rotatebox[origin=c]{90}{\bfseries 30000\strut}
\begin{subfigure}{.3\textwidth}
  \centering
  \caption{IDHC}
  % include first image
  \includegraphics[width=0.475\textwidth]{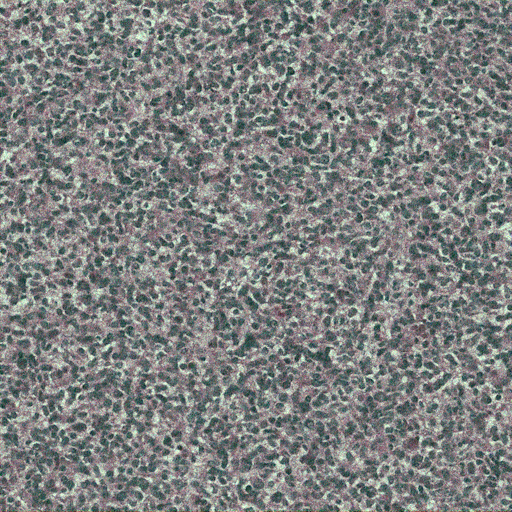} 
  % include second image
  \includegraphics[width=0.475\textwidth]{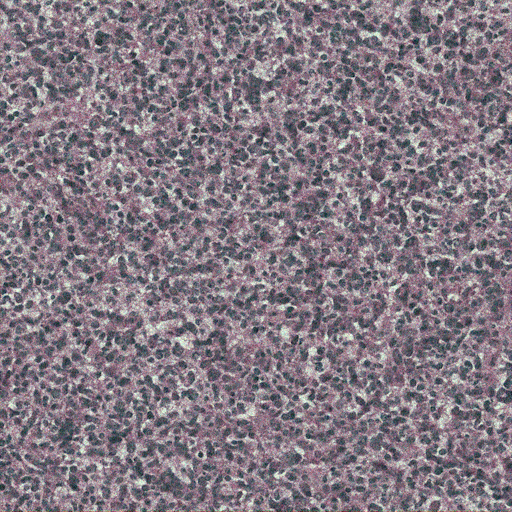}
\end{subfigure}
\begin{subfigure}{.3\textwidth}
  \centering
  \caption{IDHNC}
  % include third image
  \includegraphics[width=0.475\textwidth]{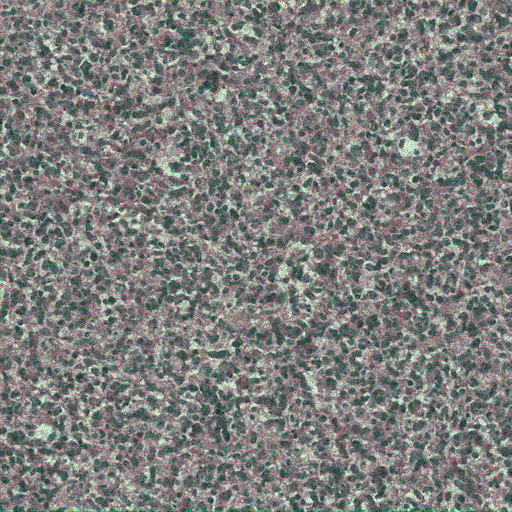} 
  % include fourth image
  \includegraphics[width=0.475\textwidth]{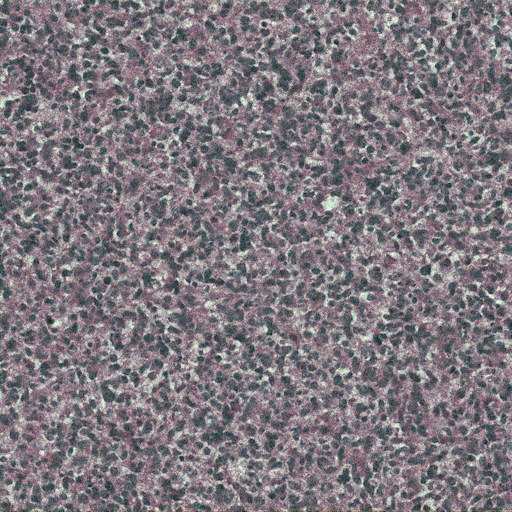}
\end{subfigure}
\begin{subfigure}{.3\textwidth}
  \centering
  \caption{IDHWT}
  % include fifth image
  \includegraphics[width=0.475\textwidth]{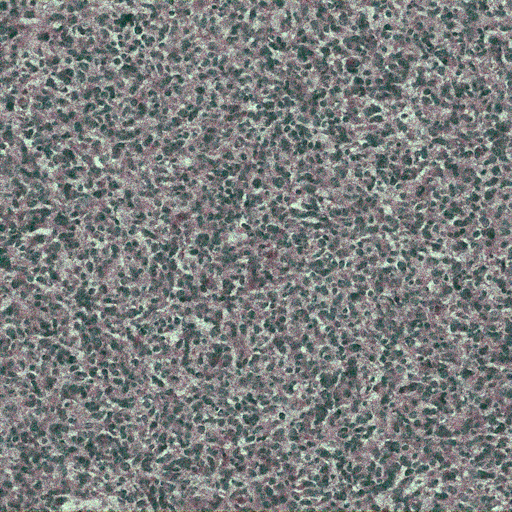} 
  % include sixth image
  \includegraphics[width=0.475\textwidth]{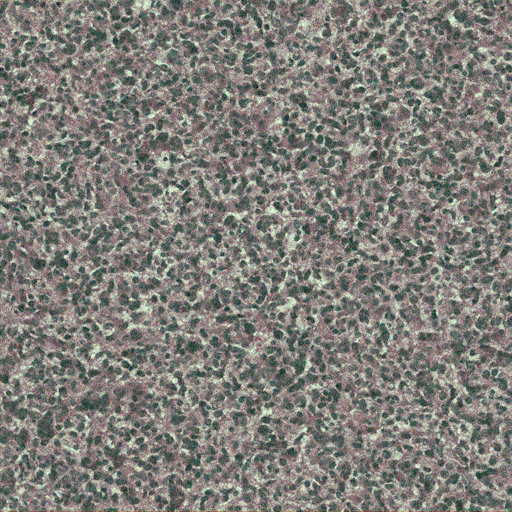}
\end{subfigure}
\newline
\rotatebox[origin=c]{90}{\bfseries 640000\strut}
\begin{subfigure}{.3\textwidth}
  \centering
  % include first image
  \includegraphics[width=0.475\textwidth]{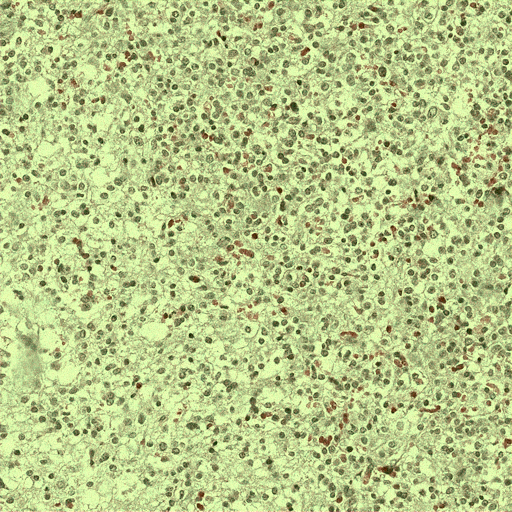} 
  % include second image
  \includegraphics[width=0.475\textwidth]{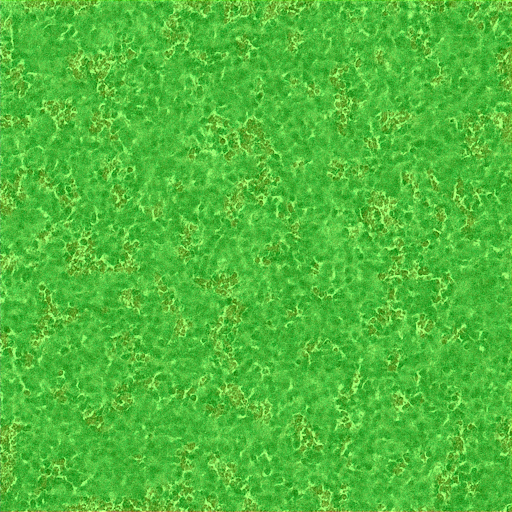}
\end{subfigure}
\begin{subfigure}{.3\textwidth}
  \centering
  % include third image
  \includegraphics[width=0.475\textwidth]{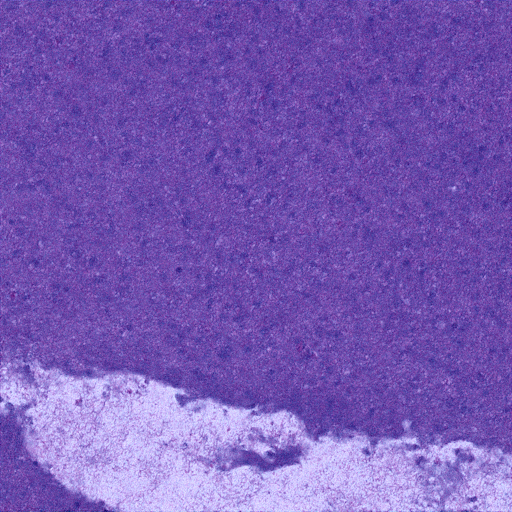} 
  % include fourth image
  \includegraphics[width=0.475\textwidth]{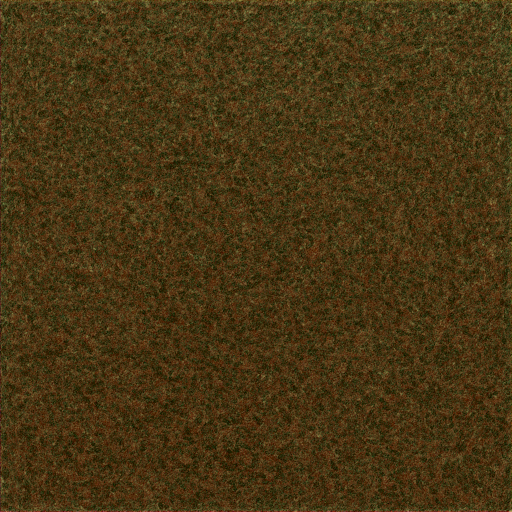}
\end{subfigure}
\begin{subfigure}{.3\textwidth}
  \centering
  % include fifth image
  \includegraphics[width=0.475\textwidth]{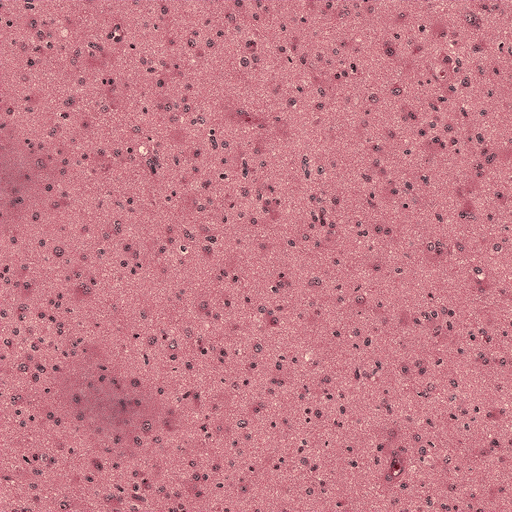} 
  % include sixh image
  \includegraphics[width=0.475\textwidth]{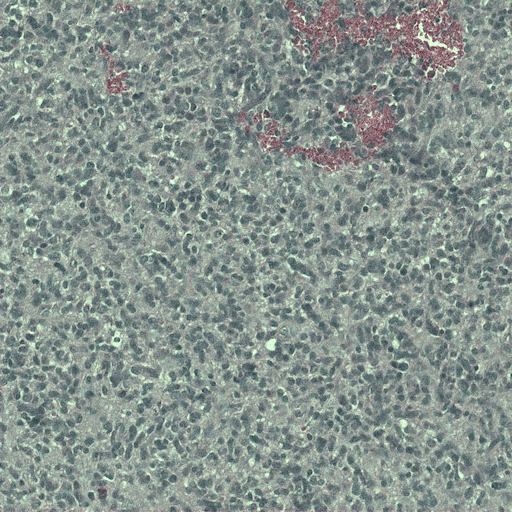}
\end{subfigure}
\caption{Selection of generated patches with DPM2. Different rows represent different steps. Each two columns together show the generated samples representing the three different subtypes of low-grade gliomas, namely IDHC, IDHNC and IDHWT.}
\label{fig:images-DPM2}
\end{figure*}
